# Supplementary material for: Learning and Type Compatibility in Signaling Games
Source: arXiv:1702.01819 ancillary file (2018-06-30)
Supplement: Supplementary file 1 [file Online_Appendix.pdf]

# Online Appendix for
# "Learning and Type Compatibility in Signalling Games"

Drew Fudenberg* Kevin He†

First version: October 12, 2016
This version: August 9, 2017

*Department of Economics, MIT. Email: drew.fudenberg@gmail.com
†Department of Economics, Harvard University. Email: hesichao@gmail.com

# OA 1 A Sufficient Condition for Type Compatibility

The definition of $\theta' \succ_{s'} \theta''$ is phrased in terms of the weakly and strictly optimal signals for types $\theta'$ and $\theta''$ against some receiver strategy $\pi_2 \in \Pi_2$, without making explicit reference to the types' payoff structures. In this section of the Online Appendix, we present a sufficient condition for type compatibility that can be directly verified from the signalling game payoff matrices.

**Definition OA.1.** For $h \in [0,1]$, the maximum and minimum *payoff wedges between types* $\theta', \theta''$ *at signal* $s'$ *with* $h$ *scaling* are

$$\overline{W}_h(\theta', \theta''; s') := \max_{a \in A} \left( (1-h) u_1(\theta', s', a) - h u_1(\theta'', s', a) \right)$$

and

$$\underline{W}_h(\theta', \theta''; s') := \min_{a \in A} \left( (1-h) u_1(\theta', s', a) - h u_1(\theta'', s', a) \right)$$

respectively.

**Proposition OA.1.** *If there exists* $h \in [0,1]$ *with*

$$\underline{W}_h(\theta', \theta''; s') > \max_{s'' \neq s'} \overline{W}_h(\theta', \theta''; s''),$$

*then* $\theta' \succ_{s'} \theta''$.

To understand the sufficient condition in Proposition OA.1, suppose we take $h = \frac{1}{2}$. Then the condition is equivalent to requiring that

$$\min_{a \in A} \left( u_1(\theta', s', a) - u_1(\theta'', s', a) \right) > \max_{s'' \neq s'} \left\{ \max_{a \in A} \left( u_1(\theta', s'', a) - u_1(\theta'', s'', a) \right) \right\}. \tag{1}$$

This says that the minimum payoff difference between type $\theta'$ and type $\theta''$ at signal $s'$ is larger than the maximum payoff difference at any other signal $s''$, where the minimum and maximum are taken over all possible receiver responses. In signalling games with separable sender payoffs $u_1(\theta, s, a) = v(\theta, s) + z(a)$, Equation (1) reduces to the sufficient condition stated in the main text,

$$v(\theta', s') - v(\theta'', s') > \max_{s'' \neq s'} \left( v(\theta', s'') - v(\theta'', s'') \right).$$

Different values of $h$ correspond to different rescalings of sender's payoffs. For each collection of $\{\alpha_\theta, \beta_\theta\}_{\theta \in \Theta}$ with $\alpha_\theta > 0$ for each $\theta$, the rescaling

$$\tilde{u}_S(\theta, s, a) \coloneqq \alpha_\theta \cdot u_1(\theta, s, a) + \beta_\theta$$

does not change any type's preference on lotteries over $(s, a)$ pairs or experimentation incentives. Substituting the rescaled payoffs into (1), we get

$$\min_{a \in A} \left( \alpha_{\theta'} u_1(\theta', s^{'}, a) - \alpha_{\theta''} u_1(\theta^{''}, s^{'}, a) \right) > \max_{s'' \neq s'} \max_{a \in A} \left( \alpha_{\theta'} u_1(\theta', s^{''}, a) - \alpha_{\theta''} u_1(\theta^{''}, s^{''}, a) \right).$$

This is equivalent to requiring $\underline{W}_h(\theta^{'}, \theta^{''}; s^{'}) > \max_{s'' \neq s'} \overline{W}_h(\theta^{'}, \theta^{''}; s^{''})$ for $h = \frac{\alpha_{\theta'}}{\alpha_{\theta'} + \alpha_{\theta''}}$.

*Proof.* **Case 1**: $h = 0$.

Then $\underline{W}_h(\theta^{'}, \theta^{''}; s^{'}) > \max_{s'' \neq s'} \overline{W}_h(\theta^{'}, \theta^{''}; s^{''})$ is equivalent to

$$\min_{a \in A} u_1(\theta^{'}, s^{'}, a) > \max_{s'' \neq s'} \max_{a \in A} u_1(\theta^{'}, s^{''}, a).$$

This means for any $\pi_2 \in \Pi_2$, $s^{'}$ is always strictly optimal for $\theta^{'}$. This shows $\theta^{'} \succ_{s'} \theta^{''}$.

**Case 2**: $h = 1$.

Then $\underline{W}_h(\theta^{'}, \theta^{''}; s^{'}) > \max_{s'' \neq s'} \overline{W}_h(\theta^{'}, \theta^{''}; s^{''})$ is equivalent to

$$\min_{a \in A} -u_1(\theta^{''}, s^{'}, a) > \max_{s'' \neq s'} \max_{a \in A} -u_1(\theta^{''}, s^{''}, a),$$

which rearranges to

$$\max_{a \in A} u_1(\theta^{''}, s^{'}, a) < \min_{s'' \neq s'} \min_{a \in A} u_1(\theta^{''}, s^{''}, a).$$

Then we vacuously have $\theta^{'} \succ_{s'} \theta^{''}$, since $s^{'}$ is never weakly optimal for $\theta^{''}$ against any $\pi_2 \in \Pi_2$.

**Case 3**: $0 < h < 1$.

Let any $\pi_2 \in \Pi_2$ that makes $s^{'}$ weakly optimal for $\theta^{''}$ be given. For any $s^{''} \neq s^{'}$, we show

$$u_1(\theta^{'}, s^{'}, \pi_2(\cdot|s^{'})) > u_1(\theta^{'}, s^{''}, \pi_2(\cdot|s^{''})).$$

From $\underline{W}_h(\theta^{'}, \theta^{''}; s^{'}) > \max_{s'' \neq s'} \overline{W}_h(\theta^{'}, \theta^{''}; s^{''})$, we get

$$(1-h)u_1(\theta^{'}, s^{'}, \pi_2(\cdot|s^{'})) - hu_1(\theta^{''}, s^{'}, \pi_2(\cdot|s^{'})) > (1-h)u_1(\theta^{'}, s^{''}, \pi_2(\cdot|s^{''})) - hu_1(\theta^{''}, s^{''}, \pi_2(\cdot|s^{''})).$$

Using the fact that $0 < h < 1$, we can rearrange this inequality as

$$u_1(\theta^{'}, s^{'}, \pi_2(\cdot|s^{'})) - u_1(\theta^{'}, s^{''}, \pi_2(\cdot|s^{''})) > \frac{h}{1-h} \cdot \left[u_1(\theta^{''}, s^{'}, \pi_2(\cdot|s^{'})) - u_1(\theta^{''}, s^{''}, \pi_2(\cdot|s^{''}))\right].$$

When $s^{'}$ is weakly optimal for $\theta^{''}$, $u_1(\theta^{''}, s^{'}, \pi_2(\cdot|s^{'})) - u_1(\theta^{''}, s^{''}, \pi_2(\cdot|s^{''})) \geq 0$. This shows $u_1(\theta^{'}, s^{'}, \pi_2(\cdot|s^{'})) - u_1(\theta^{'}, s^{''}, \pi_2(\cdot|s^{''})) > 0$, that is $s^{'}$ is strictly better than $s^{''}$ for $\theta^{'}$. Since the choice of $s^{''} \neq s^{'}$ was arbitrary, $s^{'}$ must be strictly optimal for $\theta^{'}$. We therefore conclude $\theta^{'} \succ_{s^{'}} \theta^{''}$. □

# OA 2 The Set of Steady State Strategy Profiles is Nonempty and Compact

Recall that $\Psi^*(g, \delta, \gamma)$ denotes the set of steady states under regular prior $g$, patience $0 \leq \delta < 1$, and survival chance $0 \leq \gamma < 1$, while $\Pi^*(g, \delta, \gamma)$ is the set of steady state strategy profiles associated with the same parameters, that is $\Pi^*(g, \delta, \gamma) := \sigma\left(\Psi^*(g, \delta, \gamma)\right)$. We will prove:

**Proposition 3**. $\Pi^*(g, \delta, \gamma)$ *is non-empty and compact in the norm topology.*

*Proof.* Let regular prior $g$ and parameters $0 \leq \delta, \gamma < 1$ be given.

**Step 0**: Preliminary definitions and notation.

For two states $\psi, \hat{\psi}$, let $d(\psi, \hat{\psi})$ be the $\ell_1$ distance between them, namely

$$d(\psi, \hat{\psi}) := \left(\sum_{\theta \in \Theta} \sum_{y_\theta \in Y_\theta} |\psi_\theta(y_\theta) - \hat{\psi}_\theta(y_\theta)|\right) + \sum_{y_2 \in Y_2} |\psi_2(y_2) - \hat{\psi}_2(y_2)|.$$

This is well-defined because $Y_\theta$ and $Y_2$ are countable. Furthermore, $d(\psi, \hat{\psi}) \leq 2 \cdot (|\Theta| + 1)$ for any pair of states, since each $\psi$ is a profile of $|\Theta| + 1$ measures on countable spaces, and if $\varphi$ and $\hat{\varphi}$ are measures on a countable space $X$, then $\sum_{x \in X} |\varphi(x) - \hat{\varphi}(x)| \leq 2$ by the triangle inequality.

In the main text, we defined the one-step-forward maps $f_\theta$ and $f_2$ for different agent populations. We can also define a map $f$ from state to state, namely

$$f[\psi] := (f_\theta(\psi_\theta, \sigma_2(\psi_2))_{\theta \in \Theta}, f_2(\psi_2, (\sigma_\theta(\psi_\theta))_{\theta \in \Theta})).$$

Write $\Psi \subseteq (\times_{\theta \in \Theta} \Delta(Y_\theta)) \times \Delta(Y_2)$ for those states that assign the correct mass to each generation, that is $\psi \in \Psi$ if and only if $\psi_2\left(Y_2[t]\right) = \gamma^t(1-\gamma)$ for each $t$ and $\psi_\theta(Y_\theta[t]) = \gamma^t(1-\gamma)$

for each $\theta, t$. It is clear that $f(\Psi) \subseteq \Psi$, and that $\Psi$ is convex. We now show $f : \Psi \to \Psi$ has a fixed point.

**Step 1**: We show $f$ (restricted to $\Psi$) is continuous with respect to the metric $d$.

It suffices to show that for every $\epsilon > 0$, there exists $\zeta > 0$ so that whenever $d(\psi, \psi') < \zeta$, for every $\theta \in \Theta$ we get

$$\sum_{y_\theta \in Y_\theta} |f[\psi]_\theta(y_\theta) - f[\hat{\psi}]_\theta(y_\theta)| < \epsilon$$

and

$$\sum_{y_2 \in Y_2} |f[\psi]_2(y_2) - f[\hat{\psi}]_2(y_2)| < \epsilon.$$

We will only give details for bounding $\sum_{y_\theta \in Y_\theta} |f[\psi]_\theta(y_\theta) - f[\hat{\psi}]_\theta(y_\theta)|$, since bounding $\sum_{y_2 \in Y_2} |f[\psi]_2(y_2) - f[\hat{\psi}]_2(y_2)|$ involves an exactly analogous argument.

Since $\gamma < 1$, we may find a large enough $T$ so that

$$\sum_{t=T+1}^{\infty} \gamma^t < \epsilon/4.$$

Write $G = \sum_{t=0}^{T} |Y_\theta[t]| < \infty$ for the number of type $\theta$ histories with length $T$ or shorter. (Note that this is the same number for each type $\theta$). It suffices to ensure that

$$\left| f[\psi]_\theta(y_\theta) - f[\hat{\psi}]_\theta(y_\theta) \right| < \frac{\epsilon}{2G}$$

for each $y_\theta \in \bigcup_{t=0}^{T} Y_\theta[t]$. When this is satisfied,

$$\begin{aligned}
\sum_{y \in Y_\theta} |f[\psi]_\theta(y_\theta) - f[\hat{\psi}]_\theta(y_\theta)| &= \sum_{y_\theta \in \bigcup_{t=0}^{T} Y_\theta[t]} |f[\psi]_\theta(y_\theta) - f[\hat{\psi}]_\theta(y_\theta)| + \sum_{y_\theta \in \bigcup_{t=T+1}^{\infty} Y_\theta[t]} |f[\psi]_\theta(y_\theta) - f[\hat{\psi}]_\theta(y_\theta)| \\
&< \sum_{y_\theta \in \bigcup_{t=0}^{T} Y_\theta[t]} \frac{\epsilon}{2G} + \sum_{y_\theta \in \bigcup_{t=T+1}^{\infty} Y_\theta[t]} |f[\psi]_\theta(y_\theta) - f[\hat{\psi}]_\theta(y_\theta)| \\
&< \epsilon/2 + \epsilon/2 \\
&= \epsilon,
\end{aligned}$$

where the second to last step follows from the fact that both $f[\psi]_\theta$ and $f[\hat{\phi}]_\theta$ assign mass

$$\sum_{t=T+1}^{\infty} \gamma^t (1 - \gamma) < \sum_{t=T+1}^{\infty} \gamma^t < \epsilon/4$$

to $\bigcup_{t=T+1}^{\infty} Y_\theta[t]$, so their sum of pointwise differences cannot be larger than $\epsilon/2$ by the triangle inequality.

But for an arbitrary $y_\theta \in \bigcup_{t=0}^{T} Y_\theta[t]$ with the form $y_\theta = (\tilde{y}_\theta, \sigma_\theta(\tilde{y}_\theta), a)$,[1] from the definition of $f$, the inequality $\left| f[\psi]_\theta(y_\theta) - f[\hat{\psi}]_\theta(y_\theta) \right| < \frac{\epsilon}{2G}$ is equivalent to

$$\left| \psi_\theta(\tilde{y}_\theta) \cdot \gamma \cdot \sigma_2(\psi_2)(a|\sigma_\theta(\tilde{y}_\theta)) - \hat{\psi}_\theta(\tilde{y}_\theta) \cdot \gamma \cdot \sigma_2(\hat{\psi}_2)(a|\sigma_\theta(\tilde{y}_\theta)) \right| < \epsilon/2G.$$

If $d(\psi, \hat{\psi}) < \zeta$, then in particular $|\psi_\theta(\tilde{y}_\theta) - \hat{\psi}_\theta(\tilde{y}_\theta)| < \zeta$. Furthermore, for every signal $s \in S$,

$$\begin{aligned}
\left| \sigma_2(\psi_2)(a|s) - \sigma_2(\hat{\psi}_2)(a|s) \right| &= \left| \sum_{y_2 : \sigma_2(y_2)(s) = a} \psi_2(y_2) - \hat{\psi}_2(y_2) \right| \\
&\leq \sum_{y_2 : \sigma_2(y_2)(s) = a} |\psi_2(y_2) - \hat{\psi}_2(y_2)| \\
&\leq \sum_{y_2 \in Y_2} |\psi_2(y_2) - \hat{\psi}_2(y_2)| \\
&\leq d(\psi, \hat{\psi}).
\end{aligned}$$

So in particular we see that $|\sigma_2(\psi_2)(a|\sigma_\theta(\tilde{y}_\theta)) - \sigma_2(\hat{\psi}_2)(a|\sigma_\theta(\tilde{y}_\theta))|$ can also be bounded by making $d(\psi, \hat{\psi})$ sufficiently small. Since $\bigcup_{t=0}^{T} Y_\theta[t]$ is finite, we may choose a single small enough $\zeta > 0$ such that $\left| f[\psi]_\theta(y_\theta) - f[\hat{\psi}]_\theta(y_\theta) \right| < \frac{\epsilon}{2G}$ for every $y \in \bigcup_{t=0}^{T} Y_\theta[t]$.

**Step 2**: We show $\Psi$ is compact under metric $d$.

We may write $\Psi = (\times_{\theta \in \Theta} \Psi_\theta) \times \Psi_2$, decomposing it as the product of the histories of the sender types and the receiver. Here, $\Psi_\theta \subseteq Y_\theta$ is the set of measures over type-$\theta$ histories that assign the correct mass to each generation, and $\Psi_2 \subseteq \Delta(Y_2)$ is the set of measures over receiver histories that do the same. We may define metric $d_\theta$ on $\Psi_\theta$ and $d_2$ on $\Psi_2$ using the $\ell_1$ norm, analogous to the definition of $d$. Since the metric $d$ on $\Psi$ may be written as

$$d(\psi, \hat{\psi}) = \sum_{\theta \in \Theta} d_\theta(\psi_\theta, \hat{\psi}_\theta) + d_2(\psi_2, \hat{\psi}_2),$$

it must then induce the product topology on $(\times_{\theta \in \Theta} \Psi_\theta) \times \Psi_2$.

So, it suffices to prove each of $(\Psi_\theta, d_\theta)$ and $(\Psi_2, d_2)$ is compact. We do this only for $(\Psi_2, d_2)$ since the other arguments are analogous.

We may extend the metric $d_2$ to the space $\ell^1$, the collection of absolutely summable real

[1] If $y_\theta$ is not of this form, then by definition of $f$, we have $f[\psi]_\theta(y_\theta) = 0 = f[\hat{\psi}]_\theta(y_\theta)$.

number sequences,

$$\ell^1 := \left\{ (x_k)_{k=0}^{\infty} : \sum_{k=0}^{\infty} |x_k| < \infty \right\}.$$

We view $\Psi_2$ as a subset of $\ell^1$, representing members of $\Psi_2$ as infinite sequences of numbers when convenient.

It is well-known that $(\ell^1, d_2)$ is complete. Therefore, to show that $(\Psi_2, d_2)$ is compact, we need only show it is closed in $(\ell^1, d_2)$ and that it is totally bounded.

**Step 2a**: $(\Psi_2, d_2)$ is closed in $(\ell^1, d_2)$.

To show closedness, suppose we have a sequence $\left(\psi_2^{(j)}\right)_{j=0}^{\infty}$ in $\Psi_2$, which can be viewed as a sequence of sequence of real numbers, $\left((x_k^{(j)})_{k=0}^{\infty}\right)_{j=0}^{\infty}$. Suppose $\lim_{j\to\infty}(x^{(j)}) = (x^*) \in \ell^1$. We show that in fact $x^* \in \Psi_2$. First, since $\left\|x^{(j)}\right\| = 1$ for every $j$ by property of $\Psi_2$ members being distributions, we must have $\|x^*\| = 1$. Next, let $K_t \subseteq \mathbb{N}$ be the indices corresponding to histories of length $t$. For every $x^{(j)}$,

$$\sum_{k \in K_t} x_k^{(j)} = \gamma^t \cdot (1 - \gamma)$$

by definition of $\Psi_2$. But since

$$d_2(x^{(j)}, x^*) \geq \sum_{k \in K_t} |x_k^{(j)} - x_k^*| \geq \left| \sum_{k \in K_t} x_k^{(j)} - \sum_{k \in K_t} x_k^* \right|,$$

then $x^{(j)} \to x^*$ must mean $\sum_{k \in K_t} x_k^* = \gamma^t(1 - \gamma)$ also. Therefore, the $\ell^1$ limit of the sequence $x^*$ satisfies all the requirements of $\Psi_2$ and is interpretable as a valid distribution on receiver histories. This shows $(\Psi_2, d_2)$ is closed in $(\ell^1, d_2)$.

**Step 2b**: $(\Psi_2, d_2)$ is totally bounded.

Let $\epsilon > 0$ be given. We show that we can cover $\Psi_2$ with finitely many radius-$\epsilon$ open balls in $(\ell^1, d_2)$. Find a large enough $T$ so that $\sum_{t=T+1}^{\infty} \gamma^t < \epsilon/2$. Put $G = \sum_{t=0}^{T} |Y_2[t]| < \infty$ for the total number of receiver histories with length no larger than $T$. Consider the finite collection of radius-$\epsilon$ open balls in $(\ell^1, d_2)$ centered on grid points of the form

$$\left(k_1 \cdot \frac{\epsilon}{2G}, k_2 \cdot \frac{\epsilon}{2G}, ..., k_G \cdot \frac{\epsilon}{2G}, 0, 0, 0, ...\right),$$

where for each $i$, $k_i$ varies in $\{0, 1, ..., K\}$ with $K := \lceil 2G/\epsilon \rceil$. We claim every $\psi_2 \in \Psi_2$ is of distance no larger than $\epsilon$ to at least one of those grid points. Consider first the sequence $(\hat{x}_k) \in \ell^1$ constructed from $\psi_2$ by setting all coordinates after the $G$-th one to 0. There is some grid point which is within $\frac{\epsilon}{2G}$ of $(\hat{x}_k)$ in each of the first $G$ dimensions, so that the grid

point's $d_2$ distance to $(\hat{x}_k)$ is no larger than $\epsilon/2$. At the same time, $d_2(\psi_2, (\hat{x}_k)) < \epsilon/2$, since $\psi_2$ assigns mass less than $\epsilon/2$ to histories of length $T+1$ or longer, while the sequence $(\hat{x}_k)$ has a 0 in all of those tail coordinates. By the triangle inequality then, the grid point we found is within distance $\epsilon$ of $\psi_2$. This shows $(\Psi_2, d_2)$ is totally bounded.

**Step 3**: $f : \Psi \to \Psi$ has a non-empty and compact set of fixed points.

Corollary 17.56 (page 583) from Aliprantis and Border (2006) asserts that if $X$ is a non-empty, compact, convex subset of a locally convex Hausdorff space, and $f : X \to X$ is continuous, then the set of fixed points of $f$ is compact and non-empty. But $\Psi$ can be viewed as a nonempty, compact, convex subset of $(\ell^1)^{|\Theta|+1}$ (under the product topology). Since every normed space is a locally convex Hausdorff space, $(\ell^1)^{|\Theta|+1}$ is a locally convex Hausdorff space.

**Step 4**: $\sigma : \Psi \to \Pi$ is continuous.

By definition, $\Pi^*(g, \delta, \gamma) := \sigma(\Psi^*(g, \delta, \gamma))$, where $\Psi^*(g, \delta, \gamma)$ are the $f$ fixed points from **Step 3**, so it suffices to prove that $\sigma$ is continuous.

Let $\theta \in \Theta$ and $s \in S$ be given. Then

$$\begin{aligned}
\left|\sigma_\theta(\psi_\theta)(s) - \sigma_\theta(\hat{\psi}_\theta)(s)\right| &= \left|\sum_{y_\theta : \sigma_\theta(y_\theta) = s} \psi_\theta(y_\theta) - \hat{\psi}_\theta(y_\theta)\right| \\
&\leq \sum_{y_\theta : \sigma_\theta(y_\theta) = s} |\psi_\theta(y_\theta) - \hat{\psi}_\theta(y_\theta)| \\
&\leq \sum_{y_\theta \in Y_\theta} |\psi_\theta(y_\theta) - \hat{\psi}_\theta(y_\theta)| \\
&\leq d(\psi, \hat{\psi}).
\end{aligned}$$

Since this is true for every $\theta \in \Theta$, $s \in S$, and an analogous inequality holds for each $(\theta, a)$ pair for the receiver, it follows that $\sigma$ is continuous. □

# OA 3 Patiently Stable Strategy Profiles Are Perfect Bayesian Equilibria with Heterogeneous Off-Path Beliefs

In this section, we prove:

**Proposition 5**: If strategy profile $\pi^*$ is patiently stable, then it is a perfect Bayesian equi-

librium with heterogeneous off-path beliefs.

In the main text, we have already shown that a patiently stable $\pi^*$ satisfies the third condition in the definition of perfect Bayesian equilibrium with heterogeneous off-path beliefs. So it remains to show that $\pi^*$ is a Nash equilibrium.

We follow closely the proof strategy of Fudenberg and Levine (1993), who derived a contradiction via excess option values. That is, the value function evaluated at a sufficiently long history should not be much higher than the expected current-period payoff of the optimal strategy at that history, so that the option value of the agents tends to 0. But if the learning system converges to a non-Nash outcome, then in most periods some agents of some population are playing some action even though they know an alternative action has a non-negligible chance to yield strictly higher payoff. The values of such histories are bounded away from their current period payoffs, since a sufficiently patient agent could experiment to determine whether the alternative action is indeed worthwhile. This means a positive fraction of histories have an excess option value, a contradiction.

In Fudenberg and Levine (1993), this argument relies on the finite lifetime only insofar as to ensure "almost all" histories are long enough, by picking a large enough lifetime. We can achieve the analogous effect in our infinite-horizon model by picking $\gamma$ close to 1.

The first step is to establish certain lemmas from Fudenberg and Levine (1993) in an infinite-horizon setting. We use the same numbering of lemmas as in Fudenberg and Levine (1993), and indicate these by "FL."

## OA 3.1 Notations from Fudenberg and Levine (1993)

We will adapt the following notation from Fudenberg and Levine (1993):

- The subscript "$i$" refers to either a sender type $\theta$ or to the receiver. As such:
  - $y_i$ refers to either a member of $Y_\theta$ or a member of $Y_2$;
  - $\sigma_i(y_i)$ refers to either $\sigma_\theta(y_\theta)$ or $\sigma_2(y_2)$ from the main text;
  - $V_i(y_i)$ refers to either $V_\theta(y_\theta)$ or $V_2(y_2)$ from the main text.
- $a_i$ denotes a generic action at an information set. So we have $a_i \in S$ when $i$ refers to a sender type and $a_i \in A$ when $i$ refers to the receiver. We will think of the same signal sent by two different types as two different actions that lead to the same information set. Also, the same receiver response following two different signals are viewed as different actions.

- $\varsigma_i$ denotes a generic extensive-form strategy.[2] When $i$ refers to a sender type, $\varsigma_i \in S$. When $i$ refers to the receiver, $\varsigma_i \in A^S$.

- $r_i(y_i)$ is an arbitrary rule assigning an extensive-form strategy to each history of $i$.

- If $\psi$ is a steady state, then $\psi_i$ refers to the distribution on histories $Y_i$ and $\bar{\psi} := \sigma(\psi)$ is the associated aggregate play.

- $X$ is the set of nodes of the game tree while $X(\varsigma_i)$ is the subset reachable when player $i$ plays $\varsigma_i$.

- $Z$ is the set of terminal nodes of the game tree while $Z(\varsigma_i)$ is the subset reachable when player $i$ plays $\varsigma_i$.

- $p_i(x|\pi_{-i})$ is the probability that game tree node $x$ is reached when others play mixed strategy $\pi_{-i}$ (and $i$ plays according to the path that gives rise to $x$).

- $u_i(\varsigma_i|y_i) = u_i(\varsigma_i, g_i(\cdot|y_i))$ is the expected current period payoff of playing $\varsigma_i$, according to the beliefs about opponents' play after observing history $y_i$.

- $\#(h|y_i)$ and $\#(x|y_i)$ count the number of times that information set $h$ and node $x$ have been reached in history $y_i$.

- $\#(\varsigma_i|y_i)$ counts the total number of times that player $i$'s policy rule prescribed strategy $\varsigma_i$ in history $y_i$.

- $\hat{\pi}^i_{-i}(\cdot|y_i)$ is the strategy of $-i$ constructed from sample average in $y_i$. That is, if $h$ is $j$'s information set and $a$ is one of the possible actions at $h$, then $\hat{\pi}^i_j(a|y_i) := \#(a|y_i)/\#(h|y_i)$ where $0/0 := 1$

- $\hat{p}_i(x|y_i) = p_i(x|\hat{\pi}^i_{-i}(\cdot|y_i))$ is the distribution on nodes induced by the "sample average strategy" constructed from history $y_i$.

- $p_i(x|y_i) = p_i(x|g_i(\cdot|y_i))$ is the distribution on nodes induced by the Bayesian posterior after history $y_i$

- $P(\varsigma_i, \epsilon, y_i)$ is the posterior probability given history $y_i$ that another strategy $\varsigma_i^{'}$ improves on $\varsigma_i$ by at least $\epsilon$ in expected payoff against the opponents' strategy $\pi_{-i}$. More precisely,

$$P(\varsigma_i, \epsilon, y_i) := \max_{\varsigma_i^{'}} g_i\left[\pi_{-i} : u_i(\varsigma_i^{'}, \pi_{-i}) \geq u_i(\varsigma_i, \pi_{-i}) + \epsilon|y_i\right].$$

[2] Fudenberg and Levine (1993) uses $s_i$ instead of $\varsigma_i$ but we will reserve $s$ for a generic signal.

- $B^i_\epsilon(\pi^*_{-i})$ is the set of $-i$ strategies which induce a distribution over terminal vertices $\epsilon$-close to the distribution induced by mixed strategy $\pi^*_{-i}$. More precisely,

$$B^i_\epsilon(\pi^*_{-i}) \coloneqq \{\pi_{-i} : |p_i(z|\pi^*_{-i}) - p_i(z|\pi_{-i})| \le \epsilon \ \forall z \in Z\}.$$

- $Q^i_\epsilon(\pi^*_{-i}|y_i) \coloneqq g_i(B^i_\epsilon(\pi^*_{-i})|y_i)$ is the belief placed strategies in $B^i_\epsilon(\pi^*_{-i})$ after history $y_i$.

## OA 3.2 Adapting the Lemmas to an Infinite-Horizon Model

We note first that Fudenberg and Levine (1993)'s Lemmas A.1, A.2, B.1, B.2 and 5.4 do not make use of the finite horizon. FL93 Lemmas A.1 and A.2 are basic statistical facts used in later proofs. FL93 Lemma B.1 and B.2 show that an observer facing an i.i.d. data-generating process is unlikely to have a very biased sample when the sample size grows large. FL93 Lemma 5.4 is a direct consequence of Lemma B.2 and shows that it is unlikely that some agent (i) has played strategy $\varsigma_i$ frequently, (ii) has rarely reached some node $x$ reachable under $\varsigma_i$, and yet (iii) thinks it is likely that $x$ will be reached the next time $\varsigma_i$ is played.

We restate FL93 Lemma 5.4 below because we will make explicit use of it in proving the theorem.

**FL93 Lemma 5.4.** For all $\epsilon > 0$ and functions $\eta$ such that $\eta(n) \to 0$ as $n \to \infty$ there is an $N$ such that for all $\delta, \gamma, \psi_i, r_i$, and $\varsigma_i$,

$$\psi_i \left\{ y_i : \max_{x \in X(\varsigma_i)} \hat{p}_i(x|y_i) \cdot \eta(\#(x|y_i)) > \epsilon, \text{ and } \#(\varsigma_i|y_i) > N \right\} \le \epsilon.$$

We next show how to prove several other FL93 lemmas in an infinite-horizon setting.

**FL93 Lemma 5.2.** There exists a non-increasing function $\eta(n) \to 0$ such that for all $y_i$ and $\gamma, \delta$,

$$\begin{aligned} \max_{\varsigma_i'} u_i(\varsigma_i'|y_i) - u_i(\sigma_i(y_i)|y_i) &\le V_i(y_i) - u_i(\sigma_i(y_i)|y_i) \\ &\le \left(\frac{\delta\gamma}{1-\delta\gamma}\right) \cdot \max_{x \in X(\sigma_i(y_i))} \hat{p}(x|y_i)\eta(\#(x|y_i)). \end{aligned}$$

*Proof.* Clearly $u_i(\varsigma_i'|y_i) \le V_i(y_i)$ for each $\varsigma_i'$, since one feasible strategy after history $y_i$ is just to play $\varsigma_i'$ forever. We may write by the Bellman equation:

$$V_i(y_i) = (1-\delta\gamma)u_i(\sigma_i(y_i)|y_i) + \delta\gamma \sum_{z \in Z(\sigma_i(y_i))} p_i(z|y_i) \cdot V_i(y_i, z).$$

Straightforward algebraic manipulation gives

$$V_i(y_i) - u_i(\sigma_i(y_i)|y_i) = \frac{\delta\gamma}{1-\delta\gamma}\left(\sum_{z\in Z(\sigma_i(y_i))} p_i(z|y_i)\cdot(V_i(y_i,z) - V_i(y_i))\right).$$

The proof in Fudenberg and Levine (1993) implies

$$\sum_{z\in Z(\sigma_i(y_i))} p_i(z|y_i)\cdot(V_i(y_i,z) - V_i(y_i)) \leq U\cdot \sum_{z\in Z(\sigma_i(y_i))} p_i(z|y_i)\cdot \parallel g_i(\cdot|(y_i,z) - g_i(\cdot|y_i) \parallel_1$$

and

$$p_i(z|y_i)\cdot \parallel g_i(\cdot|(y_i,z) - g_i(\cdot|y_i) \parallel_1 < 2\int \parallel p_i(z|\pi_{-i}) - \hat{p}_i(z|y_i) \parallel g_i(\pi_{-i}|y_i)d\pi_{-i},$$

where $U$ is maximal difference between two payoffs in the game and $\| \cdot \|_1$ is the $L_1$ norm. But by FL93 Lemma B.1, for every $z$,

$$\int \parallel \; p_i(z|\pi_{-i}) - \hat{p}_i(z|y_i) \parallel g_i(\pi_{-i}|y_i)d\pi_{-i} < \max_{x\in X(\varsigma_i)} \hat{p}_i(x|y_i)\eta(\#(x|y_i)),$$

so now modify $\eta$ from FL93 Lemma B.1 by dividing it by $2U$ times the number of terminal vertices. □

**FL93 Lemma 5.3**. For all $0<\epsilon<1$ and $\Delta > 0$, there is $\underline{\beta} < 1$ such that for all $y_i$ if $\delta\gamma > \underline{\beta}$, then

$$\Delta\cdot P(\sigma_i(y_i),\Delta,y_i) - \epsilon \leq \frac{V_i(y_i) - u_i(\sigma_i(y_i)|y_i)}{1-\epsilon}.$$

*Proof.* As in Fudenberg and Levine (1993), let $\bar{U}$ be the largest absolute payoff of the game (set to 1 if less than 1). Using their "$t$-period hypothesis testing" policy, according to their arguments we get utility of at least

$$-(1-(\delta\gamma)^t)\bar{U} + (\delta\gamma)^t\cdot\left[u_i(\sigma_i(y_i),y_i) + (1-\epsilon/2\bar{U})\Delta\cdot P(\sigma_i(y_i),\Delta,y_i) - \epsilon/2\right] \leq V_i(y_i).$$

Doing the same algebraic manipulations as in Fudenberg and Levine (1993) gives

$$\Delta\cdot P(\sigma_i(y_i),\Delta,y_i) \leq \frac{(1-(\delta\gamma)^t)\bar{U} + \epsilon/2}{(\delta\gamma)^t(1-\epsilon/2\bar{U})} + \frac{1}{1-(\epsilon/2\bar{U})}\left[V_i(y_i) - u_i(\sigma_i(y_i)|y_i)\right].$$

As $\delta\gamma \to 1$, this bound approaches

$$\Delta\cdot P(\sigma_i(y_i),\Delta,y_i) \leq \frac{\epsilon/2}{(1-\epsilon/2\bar{U})} + \frac{1}{1-(\epsilon/2\bar{U})}\left[V_i(y_i) - u_i(\sigma_i(y_i)|y_i)\right],$$

which implies

$$\frac{(1-\epsilon/2\bar{U})}{1-\epsilon}\Delta \cdot P(\sigma_i(y_i),\Delta,y_i) \le \frac{\epsilon/2}{1-\epsilon} + \frac{V_i(y_i) - u_i(\sigma_i(y_i)|y_i)}{1-\epsilon}.$$

Since $\frac{(1-\epsilon/2\bar{U})}{1-\epsilon} > 1$ and $\frac{\epsilon/2}{1-\epsilon} < \epsilon$ for small $\epsilon$, this bound implies for all small enough $\epsilon$,

$$\Delta \cdot P(\sigma_i(y_i),\Delta,y_i) - \epsilon \le \frac{V_i(y_i) - u_i(\sigma_i(y_i)|y_i)}{1-\epsilon}.$$

So there exists $\underline{\beta} < 1$ such that whenever $\delta\gamma > \underline{\beta}$ and $\epsilon$ is sufficiently small, the lemma obtains. But if the lemma obtains for $\epsilon'$, then it also obtains for any $\epsilon > \epsilon'$. Therefore the lemma holds for any $0 < \epsilon < 1$. □

**FL93 Corollary 5.5.** For all $\epsilon > 0$, there exists $N$ such that for all $\delta, \gamma$,

$$\psi_i \left\{ y_i : V_i(y_i) - u_i(\sigma_i(y_i)|y_i) > \left(\frac{\delta\gamma}{1-\delta\gamma}\right) \cdot \epsilon, \text{ and } \#(\sigma_i(y_i)|y_i) > N \right\} \le \epsilon.$$

*Proof.* Since FL93 Lemma 5.4 applies to all $\varsigma_i$,

$$\psi_i \left\{ y_i : \max_{x \in X(\sigma_i(y_i))} \hat{p}_i(x|y_i) \cdot \eta(\#(x|y_i)) > \epsilon, \text{ and } \#(\sigma_i(y_i)|y_i) > N \right\} \le \epsilon.$$

Take the $\eta(n)$ implied by FL93 Lemma 5.2, which guarantees that

$$V_i(y_i) - u_i(\sigma_i(y_i)|y_i) \le \left(\frac{\delta\gamma}{1-\delta\gamma}\right) \cdot \max_{x \in X(\sigma_i(y_i))} \hat{p}(x|y_i)\eta(\#(x|y_i))$$

uniformly for all $y_i, \gamma, \delta$. Putting this $\eta(n)$ in the sharpened FL93 Lemma 5.4 and using the above inequality, we get that we can find an $N$ so that for all $\delta, \gamma$,

$$\psi_i \left\{ y_i : V_i(y_i) - u_i(\sigma_i(y_i)|y_i) > \left(\frac{\delta\gamma}{1-\delta\gamma}\right) \cdot \epsilon, \text{ and } \#(\sigma_i(y_i)|y_i) > N \right\} \le \epsilon.$$

□

**FL93 Lemma 5.6.** For all $\epsilon > 0$ there exists a $\phi > 0$ such that when the aggregate play of $-i$ is $\bar{\psi}_{-i}$ and $i$ uses policy $r_i(y_i)$, then for any discount factor $\gamma$,

$$\psi_i \left\{ y_i : Q^i_\epsilon(\bar{\psi}_{-i}|y_i)/Q^i_\epsilon(\bar{\psi}_{-i}|0) \le \phi \right\} \le \epsilon.$$

*Proof.* This depends only on FL93 Lemma B.1 and FL93 Lemma 5.4, and does not make use of the finite horizon assumption. □

**FL93 Lemma 5.7'**. Consider a steady state $\psi_i$ for survival probability $\gamma$. Then[3]

$$\psi_i\{y_i : \#(\varsigma_i|y_i) > N \text{ and } \sigma_i(y_i) = \varsigma_i\} > \bar{\psi}_i(\varsigma_i) - (1 - (\gamma)^N).$$

*Proof.* Fix $N$. For any infinite history of $i$, there exist at most $N$ finite sub-histories $y_i'$ where $\sigma_i(y_i') = \varsigma_i$ and $\#(\varsigma_i|y_i') \leq N$. These sub-histories will have the highest probabilities if they occur in the first $N$ periods of lifetime, so that

$$\psi_i\{y_i : \#(\varsigma_i|y_i) \leq N \text{ and } \sigma_i(y_i) = \varsigma_i\} < 1 - (\gamma)^N.$$

But then,

$$\begin{aligned}
\psi_i\{y_i : \#(\varsigma_i|y_i) > N \text{ and } \sigma_i(y_i) = \varsigma_i\} &= \psi_i\{y_i : \sigma_i(y_i) = \varsigma_i\} - \psi_i\{y_i : \#(\varsigma_i|y_i) \leq N \text{ and } \sigma_i(y_i) = \varsigma_i\} \\
&= \bar{\psi}_i(\varsigma_i) - \psi_i\{y_i : \#(\varsigma_i|y_i) \leq N \text{ and } \sigma_i(y_i) = \varsigma_i\} \\
&> \bar{\psi}_i(\varsigma_i) - (1 - (\gamma)^N).
\end{aligned}$$

□

## OA 3.3 Proof of Proposition 5

*Proof.* We first establish that for any fixed regular prior $g^0$ there is a function $\gamma(\delta)$ such that if $\delta_j \to 1$, $\gamma_j \geq \gamma(\delta_j)$, and $\bar{\psi}^{(j)} \in \Pi^*(g^0, \delta_j, \gamma_j)$ is a sequence of steady state strategy profiles, then any accumulation point of $(\bar{\psi}^{(j)})$ is a Nash equilibrium. As in the proof of Theorem 5.1 in Fudenberg and Levine (1993), it suffices to show that for each $\Delta > 0$, there exists a function $\gamma(\delta, \Delta)$ such that if $\delta_j \to 1$ and $\gamma_j \geq \gamma(\delta_j, \Delta)$, any accumulation point $\bar{\psi}$ of the sequence of the steady state strategies $\bar{\psi}^{(j)}$ has the property that neither the receiver nor any sender type can gain more than $3\Delta$ by deviating from $\bar{\psi}_i$. (In a signalling game where each sender type has positive probability, a strategy profile is Nash if and only if neither the receiver nor any sender type has a profitable deviation.)

Fix $\Delta > 0$. We will construct the function $\delta \mapsto \gamma(\delta, \Delta)$. Find $\underline{\beta}(\epsilon, \Delta)$ to satisfy FL93 Lemma 5.3. Fix some function $\epsilon : (0, 1) \to (0, 1)$ satisfying $\epsilon(\delta) \downarrow 0$ as $\delta \uparrow 1$, and let $\epsilon(\delta)$ tend to 0 slowly enough as $\delta \to 1$ that $\delta > \sqrt{\underline{\beta}(\epsilon(\delta), \Delta)}$ for all $\delta$ close enough to 1. Also, for each $\delta$, find $N(\delta)$ to satisfy Corollary 5.5 for $\epsilon = \frac{(1-\delta)^2}{\delta}$, so that in any steady state $\psi$ we have

$$\psi_i\left\{y_i : V_i(y_i) - u_i(\sigma_i(y_i)|y_i) > \left(\frac{\delta\gamma}{1 - \delta\gamma}\right) \cdot \frac{(1 - \delta)^2}{\delta}, \#(\sigma_i(y_i)|y_i) > N(\delta)\right\} \leq \frac{(1 - \delta)^2}{\delta}. \quad (2)$$

[3] This claim is stronger than the one in Lemma 5.7 of Fudenberg and Levine (1993) since we do not require that $\varsigma_i$ is played with positive probability in a $\delta$-stable state.

Now, choose $\gamma(\delta, \Delta)$ near enough 1 so that for each $\delta$, (i) $\delta \cdot \gamma(\delta, \Delta) > \underline{\beta}(\epsilon(\delta), \Delta)$; (ii) $1 - (\gamma(\delta, \Delta))^{N(\delta)} < 1 - \delta$.

Suppose we have a sequence $(\delta_j, \gamma_j)$ with $\delta_j \to 1$ and $\gamma_j \geq \gamma(\delta_j, \Delta)$ for every $j \in \mathbb{N}$, and $\bar{\psi}$ is a limit of steady state strategy profiles $\bar{\psi}^{(j)}$ . If some player can gain more than $3\Delta$ by playing $\varsigma_i'$ against $\bar{\psi}_{-i}$ instead of some prescribed strategy $\varsigma_i$ where $\bar{\psi}_i(\varsigma_i) > 0$, then following the same reasoning as in Fudenberg and Levine (1993), there exists $j_0$,$\epsilon_0$ so that whenever $j > j_0$, $\epsilon < \epsilon_0$, player $i$ can gain at least $\Delta$ against any profile of $i$'s opponents within $\epsilon$ of $\bar{\psi}_{-i}^{j}$ by playing $\varsigma_i'$ instead of $\varsigma_i$. So whenever $j > j_0, \epsilon < \epsilon_0$, we have

$$P(\varsigma_i, \Delta, y_i) \geq Q_\epsilon^i(\bar{\psi}_{-i}^{(j)} | y_i)$$

for every history $y_i$. We may also choose $j_0$ so that whenever $j > j_0$, $\bar{\psi}^{(j)}(\varsigma_i) > \bar{\psi}(\varsigma_i)/2$.

Picking $\epsilon = \bar{\psi}_i(\varsigma_i)/4 > 0$ in FL93 Lemma 5.6, we get that there exists a $\phi > 0$ so that

$$\psi_i^{(j)} \left\{ y_i : Q_\epsilon^i(\bar{\psi}_{-i}^{(j)} | y_i) / Q_\epsilon^i(\bar{\psi}_{-i}^{(j)} | 0) \leq \phi \right\} \leq \bar{\psi}_i(\varsigma_i)/4$$

for all $j$ and $y_i$. Therefore,

$$\psi_i^{(j)}(y_i : P(\varsigma_i, \Delta, y_i) > \phi \underline{Q}) > 1 - \bar{\psi}_i(\varsigma_i)/4$$

for all $j > j_0$, where $\underline{Q}$ is the minimum density under prior $g^0$. Note that $\underline{Q} > 0$ since $g^0$ is regular.

Using FL93 Lemma 5.7 and the fact that $1 - (\gamma_j)^{N(\delta_j)} < 1 - \delta_j$ (from (ii) in the definition of $\gamma(\delta, \Delta)$), combined with the fact $\bar{\psi}_i^{(j)}(\varsigma_i) > \bar{\psi}_i(\varsigma_i)/2$,

$$\psi_i^{(j)}\{y_i : \#(\varsigma_i | y_i) > N(\delta_j) \text{ and } \sigma_i^{(j)}(y_i) = \varsigma_i\} > \bar{\psi}_i(\varsigma_i)/2 - (1 - \delta_j).$$

So then

$$\begin{aligned} \psi_i^{(j)}(y_i : P(\varsigma_i, \Delta, y_i) > \phi \underline{Q}, \#(\varsigma_i | y_i) > N(\delta_j) \text{ and } \sigma_i^{(j)}(y_i) = \varsigma_i) &> \left[\bar{\psi}_i(\varsigma_i)/2 - (1 - \delta_j)\right] - \left[\bar{\psi}_i(\varsigma_i)/4\right] \\ &= \bar{\psi}_i(\varsigma_i)/4 - (1 - \delta_j) \qquad (3) \end{aligned}$$

for every $j > j_0$. Now using the fact that $\delta_j \cdot \gamma_j > \underline{\beta}(\epsilon(\delta_j), \Delta)$ from (i) in the definition of $\gamma(\delta, \Delta)$, after every history $y_i$,

$$\Delta \cdot P(\sigma_i(y_i), \Delta, y_i) - \epsilon(\delta_j) \leq \frac{V_i(y_i) - u_i(\sigma_i^{(j)}(y_i) | y_i)}{1 - \epsilon(\delta_j)}$$

by FL93 Lemma 5.3. Combining this with (3), we have

$$\psi_i^{(j)}\left(y_i : \begin{array}{c}[V_i(y_i) - u_i(\sigma_i(y_i)|y_i) > (\Delta\phi\underline{Q} - \epsilon(\delta_j)) \cdot (1 - \epsilon(\delta_j))],\\ \#(\varsigma_i|y_i) > N(\delta_j), \text{ and } \sigma_i^{(j)}(y_i) = \varsigma_i\end{array}\right) > \bar{\psi}_i(\varsigma_i)/4 - (1 - \delta_j).$$

By choosing large enough $j$, we may ensure that $(\Delta\phi\underline{Q} - \epsilon(\delta_j)) \cdot (1 - \epsilon(\delta_j)) > 1 - \delta_j$ and also that $\bar{\psi}_i(\varsigma_i)/4 - (1 - \delta_j) > \frac{(1-\delta_j)^2}{\delta_j}$. But at such large enough $j$,

$$\psi_i^j(y_i : [V_i(y_i) - u_i(\sigma_i(y_i)|y_i) > 1 - \delta_j], \#(\varsigma_i|y_i) > N(\delta_j), \text{ and } \sigma_i^{(j)}(y_i) = \varsigma_i) > \frac{(1-\delta_j)^2}{\delta_j}.$$

This contradicts (2), because $\left(\frac{\delta_j\gamma_j}{1-\delta_j\gamma_j}\right) \cdot \frac{(1-\delta_j)^2}{\delta_j} \leq \left(\frac{\delta_j}{1-\delta_j}\right) \cdot \frac{(1-\delta_j)^2}{\delta_J} = 1 - \delta_j$.

Having established the existence of the function $\gamma(\delta, \Delta)$, we can now prove Proposition 5. Suppose $\bar{\psi}$ is patiently stable. Then we can find $\delta_j \to 1$, a sequence $(\bar{\psi}^{(j)})$ such that $\bar{\psi}^{(j)}$ is $\delta_j$-stable for each $j$ and $\lim_{j\to\infty} \bar{\psi}^{(j)} = \bar{\psi}$. For each $j$, there corresponds a sequence $\gamma_{j,k} \to 1$ and a sequence of steady state strategy profiles $\bar{\psi}^{j,k} \in \Pi^*(g^0, \delta_j, \gamma_{j,k})$ such that $\lim_{k\to\infty} \bar{\psi}^{(j,k)} = \bar{\psi}^{(j)}$. Find the function $\gamma(\delta, \Delta)$ implied by the above argument. For each $j$, pick $k(j)$ large enough so that $\gamma_{j,k(j)} > \gamma(\delta_j, \Delta)$ and $\bar{\psi}^{j,k(j)}$ is less than $1/j$ away from $\bar{\psi}^j$. Then by construction of $(\delta_j, \gamma_{j,k(j)}, \bar{\psi}^{j,k(j)})$, every accumulation point of the sequence $(\bar{\psi}^{j,k(j)})$ is a Nash equilibrium. But $\bar{\psi}$ is the limit point of this sequence. □

# OA 4 $\delta$-Stable Strategy Profiles Are Type-Heterogeneous Self-Confirming Equilibria

**Proposition 4**: Suppose strategy profile $\pi^*$ is $\delta$-stable under a regular prior. Then for every type $\theta$ and signal $s$ with $\pi_1^*(s|\theta) > 0$, $s$ is a best response to some $\pi_2 \in \Pi_2$ for type $\theta$, and furthermore $\pi_2(\cdot|s) = \pi_2^*(\cdot|s)$. Also, for any signal $s$ such that $\pi_1^*(s|\theta) > 0$ for at least one type $\theta$, $\pi_2^*(\cdot|s)$ is supported on pure best responses to the Bayesian belief generated by $\pi_1^*$ after $s$.

*Proof.* **Step 1**: We first show that for every $s$ with $\pi_1^*(s|\theta) > 0$ for at least one type $\theta$, $\pi_2^*(\cdot|s)$ is supported on pure best responses to the Bayesian belief generated by $\pi_1^*$ after $s$, namely $p^*(\theta|s) := \frac{\lambda(\theta)\cdot\pi_1^*(s|\theta)}{\sum_{\theta'}\lambda(\theta')\cdot\pi_1^*(s|\theta')}$.

Suppose $a$ is not a best response to $p^*(\cdot|s)$ after $s$. Since $\pi_1^*(s|\theta)$ is nonzero for at least one type $\theta$, there must exist $\epsilon > 0$ such that $a$ is also not a best response to any belief $p^{'}(\cdot|s)$

generated by

$$p^{'}(\theta|s)=\frac{\lambda(\theta)\cdot\pi^{'}(s|\theta)}{\sum_{\theta'}\lambda(\theta')\cdot\pi^{'}(s|\theta')}$$

whenever $|\pi_{\theta}^{*}(s)-\pi_{\theta}^{'}(s)|<\epsilon$ for every $s$.

Fixing arbitrary $\Delta>0$, we now show $\pi_2^*(a|s)<\Delta$. Take a sequence of steady states $\psi^k\in\Psi^*(g,\delta,\gamma_k)$ for $\gamma_k\to 1$ such that $\bar{\psi}^k\to\pi^*$. We now make use of FL Lemma B.1, which (in our notation) states that for every regular prior $g$, there exists a non-increasing function $\eta(n)\to 0$ as $n\to\infty$, such that for every receiver history $y_2$ we get

$$\int_{\Pi_1}\parallel\pi_1(s|\theta)-\frac{\#(\theta,s|y_2)}{\#(\theta|y_2)}\parallel g_2(\pi_1|y_2)d\pi_1<\eta(\#(\theta|y_2)),$$

where $\#(\theta|y_2)$ counts the number of times that the receiver has encountered type $\theta$'s in history $y_2$ and $\#(\theta,s|y_2)$ counts the number of times that type $\theta$'s played signal $s$ in history $y_2$. Find a large enough $N_1\in\mathbb{N}$ such that $\eta(N_1)<\epsilon/3$ and a large enough $N_2$ such that

$$\mathbb{P}\left[|(B_{n,p}/n)-p|>\epsilon/3\right]<\Delta/(3\cdot|\Theta|)$$

for all $p\in[0,1]$ and $n\geq N_2$, where $B_{n,p}\sim\text{Binom}(n,p)$. Find next a large enough $N_3$ so that after $n\geq N_3$ periods, a receiver will have encountered $\max(N_1,N_2)$ instances of each type of sender with probability at least $1-\Delta/3$.

Find now a large enough $K$ so that whenever $k\geq K$ we have $|\bar{\psi}_1^{(k)}(s|\theta)-\pi^*(s|\theta)|<\epsilon/3$ for each $\theta$. We claim that whenever $k\geq K$, each receiver in $\psi^k$ older than $N_3$ has less than a $2\Delta/3$ chance of playing action $a$ after signal $s$. This is because there is less than $\Delta/3$ chance that the receiver has not seen at least $\max(N_1,N_2)$ instances of each type of sender. In the event that he has, there is a further $\Delta/3$ chance that the empirical frequency of any one type playing $s$ deviates more than $\epsilon/3$ from its data-generating frequency $\bar{\psi}_1^k(s|\theta)$. Otherwise, B.1 of Fudenberg and Levine (1993) guarantees that the receiver's posterior mean probability of $\theta$ playing $s$ is no more than $2\epsilon/3$ away from $\bar{\psi}_1^k(s|\theta)$, which is in turn no more than $\epsilon/3$ away from $\pi_1^*(s|\theta)$. But we have defined $\epsilon$ such that under this belief, $a$ is not a best response. As we take large enough $k$, the fraction of individuals aged $N_3$ or younger tends to 0, so in particular there must be in total fewer than $\Delta$ fraction of receivers playing $a$ after $m$.

**Step 2**: We show that if $\pi_1^*(s|\theta)>0$, then $s$ is a best response for type $\theta$ to some $\pi_2\in\Pi_2$ where $\pi_2(\cdot|s)=\pi_2^*(\cdot|s)$. We prove the contrapositive and suppose $s$ is not a best response to any $\pi_2\in\tilde{\Pi}_2$, where $\tilde{\Pi}_2\subseteq\Pi_2$ is the subset of behavior receiver strategies that agree with $\pi_2^*$ after $s$,

$$\tilde{\Pi}_2:=\{\pi_2\in\Pi_2:\pi_2(\cdot|s)=\pi_2^*(\cdot|s)\}.$$

Since $s$ does not best respond to $\tilde{\Pi}_2$ for type $\theta$ and since $\tilde{\Pi}_2$ is compact, there exists some $2\xi > 0$ so that $s$ is not a $2\xi$ best response to any strategy in $\tilde{\Pi}_2$. Fix such an $\xi$, and fix a small enough $r > 0$ such that $s$ is not a $\xi$ best response to any strategy in $\Pi_2$ no further than $r$ away from $\tilde{\Pi}_2$ in the $\ell_1$ norm. Call the set of such strategies $\tilde{\tilde{\Pi}}_2$.

Find the function $\eta(n) \to 0$ corresponding to FL93 Lemma 5.2. Choose any $\epsilon > 0$ small enough such that $\frac{1}{1-\frac{1}{2}\delta} \cdot \epsilon < \xi$. We will show that for $k$ large enough, $\bar{\psi}_1^k(s|\theta) < 4\epsilon$. This would show that $\pi_1^*(s|\theta) < 4\epsilon$ for all small enough $\epsilon$, so $\pi_1^*(s|\theta) = 0$ as desired.

To proceed, first note that by the choice of $\epsilon$ small enough, at every history $y_\theta$ where

$$\max_{\hat{s}} \left(u_\theta(\hat{s}|y_\theta) - u_\theta(s|y_\theta)\right) > \xi,$$

we would also have

$$\max_{\hat{s}} \left(u_\theta(\hat{s}|y_\theta) - u_\theta(\sigma_\theta(y_\theta)|y_\theta)\right) > \frac{1}{1-\frac{1}{2}\delta} \cdot \epsilon \geq \frac{\delta\gamma_k}{1-\delta\gamma_k}\epsilon$$

whenever $\gamma_k \geq \frac{1}{2}$. But the choice of $\eta(n) \to 0$ ensures that, by FL93 Lemma 5.2,

$$\max_{\hat{s}} \left(u_\theta(\hat{s}|y_\theta) - u_\theta(\sigma_\theta(y_\theta)|y_\theta)\right) \leq \frac{\delta\gamma_k}{1-\delta\gamma_k} \max_{x\in X(\sigma_\theta(y_\theta))} \hat{p}(x|y_\theta)\eta(\#(x|y_\theta)).$$

Hence, we conclude that whenever both $\sigma_\theta(y_\theta) = s$ and $\max_{\hat{s}} \left(u_\theta(\hat{s}|y_\theta) - u_\theta(s|y_\theta)\right) > \xi$, we have $\max_{x\in X(m)} \hat{p}(x|y_\theta)\eta(\#(x|y_\theta)) > \epsilon$.

But now by FL93 Lemma 5.4, there exists $N \in \mathbb{N}$ so that

$$\psi_\theta^k \left\{ y_\theta : \max_{x\in X(s)} \hat{p}(x|y_\theta)\eta(\#(x|y_\theta)) > \epsilon \text{ and } \#(s|y_\theta) > N \right\} \leq \epsilon.$$

This shows that at most fraction $\epsilon$ of the histories satisfy the following the requirements that:

(1) $\theta$ is playing $s$;

(2) $\theta$ has played $s$ at least $N$ times; and

(3) $s$ is not a $\xi$ myopic best response for $\theta$,that is

$$\psi_\theta^k \left\{ y_\theta : \sigma_\theta(y_\theta) = s, \#(s|y_\theta) > N, \max_{\hat{s}} \left(u_\theta(\hat{s}|y_\theta) - u_\theta(s|y_\theta)\right) > \xi \right\} \leq \epsilon.$$

Therefore, histories at which $\theta$ is allowed to play $s$ fall into at least one of the following three categories:

**Exception 1**: The set described above, with a mass no larger than $\epsilon$.

**Exception 2**: Histories where $\sigma_\theta(y_\theta) = s$ but $\#(s|y_\theta) \leq N$. There can be no more than $N$ such periods in any sender's life, so then this exception accounts for mass less than

$(1-\gamma_k)\cdot N$. There exists $K_1$ such that $(1-\gamma_k)\cdot N<\epsilon$ for all $k\geq K_1$.

**Exception 3**: Histories where $s$ is a myopic $\xi$ best response to $\pi_2(\cdot|y_\theta)$, the expected receiver strategy under the sender's posterior $g_1(\cdot|y_\theta)$ . We will show that these histories have mass no larger than $2\epsilon$.

To do so, apply FL93 Lemma B.1, to find function $\hat{\eta}(n)\to 0$ such that for every $a\in A$,

$$\int_{\Pi_2} \parallel \pi_2(a|s)-\frac{\#(s,a|y_\theta)}{\#(s|y_\theta)} \parallel g_1(\pi_2|y_\theta)d\pi_2<\hat{\eta}(\#(s|y_\theta)).$$

So, there exists $N_1\in\mathbb{N}$ such that whenever $\#(s|y_\theta)>N_1$, $\pi_2(\cdot|s;y_\theta)$ is no more than $r/3$ away in $\ell_1$ norm from $\hat{\pi}_2(\cdot|s;y_\theta)$, where $\hat{\pi}_2$ is the receiver strategy formed by the empirical distribution in $y_\theta$.

But for each $k$, the strong law of large numbers implies there exists some $N_2\in\mathbb{N}$ such that the $\hat{\pi}_2(\cdot|s)$ based on empirical frequency will not differ too much from the data-generating $\bar{\psi}_2^k(\cdot|s)$ given more than $N_2$ observations:

$$\psi_\theta^k\left\{y_\theta : d(\hat{\pi}_2(\cdot|s;y_\theta),\bar{\psi}_2^k(\cdot|s))>r/3, \#(s|y_\theta)>N_2\right\}<\epsilon,$$

where $d$ denotes the distance in $\ell_1$ norm. Finally, since $\lim_{k\to\infty}\bar{\psi}_2^k=\pi_2^*$, there is $K_2$ such that $k\geq K_2$ implies

$$d(\pi_2^*(\cdot|s),\bar{\psi}_2^k(\cdot|s))<r/3.$$

But then, by the triangle inequality, whenever $k\geq K_2$ we have

$$\psi_\theta^k\left\{y_\theta : [d(\pi_2^*(\cdot|s),\pi_2(\cdot|s;y_\theta))<r] \text{ and } [\#(s|y_\theta)>\max(N_1,N_2)]\right\}\leq\epsilon.$$

Now whenever $d(\pi_2^*(\cdot|s),\pi_2(\cdot|s;y_\theta))<r$, $\pi_2$ must be no more than $r$ distance away from $\tilde{\tilde{\Pi}}_2$, the set of receiver strategies that differ by no more than $r$ from $\pi_2^*$ at signal $s$. Recall that $\tilde{\tilde{\Pi}}_2$ has the property that $s$ is not even a $\xi$ best response to any of the strategies in it. So, we have shown whenever $k_2\geq K$,

$$\psi_\theta^k\left\{y_\theta : \#(s|y_\theta)>\max(N_1,N_2), \max_{\hat{s}}\left(u_\theta(\hat{s}|y_\theta)-u_\theta(s|y_\theta)\right)\leq\xi\right\}\leq\epsilon.$$

But, we may find $K_3$ such that $k\geq K_3$ implies

$$\psi_\theta^k\left\{y_\theta : \#(s|y_\theta)\leq\max(N_1,N_2)\right\}\leq\epsilon.$$

Therefore, provided $k\geq\max(K_2,K_3)$, exception 3 accounts for no more than $2\epsilon$ of the histories.

Now find $K_4$ such that $k \geq K_4$ implies $\gamma_k \geq \frac{1}{2}$. We have therefore shown whenever $k \geq \max(K_1, K_2, K_3, K_4)$, that the set of histories $y_\theta$ where $\sigma_\theta(y_\theta) = s$ has $\psi_\theta^k$ mass no larger than $4\epsilon$, as desired. □

# OA 5 Proof of Lemma 3

**Lemma 3**: Fix a regular prior $g$ and a strategy profile $\pi^*$ where for some type $\theta'$ and signal $s^{'}$, $\theta^{'} \in J(s^{'}, \pi^*)$.

There exist a number $\epsilon$ and functions $N \mapsto \delta(N)$ and $(N, \delta) \mapsto \gamma(N, \delta)$, all valued in $(0, 1)$, such that whenever:

- $\delta \geq \delta(N)$, $\gamma \geq \gamma(N, \delta)$
- $\pi \in \Pi^*(g, \delta, \gamma)$
- $\pi$ is no further away than $\epsilon$ from $\pi^*$ in $\ell_1$ norm

we have $\pi_1(s^{'}|\theta^{'}) \geq (1 - \gamma) \cdot N$.

By $\ell_1$ norm we mean the norm generated by the metric

$$d(\pi, \pi^*) = \sum_{\theta \in \Theta} \sum_{s \in S} |\pi_1(s|\theta) - \pi_1^*(s|\theta)| + \sum_{s \in S} \sum_{a \in A} |\pi_2(a|s) - \pi_2^*(a|s)|.$$

*Proof.* Let $g, \pi^*, \theta^{'}, s^{'}$ satisfying the hypotheses of the lemma be given.

Find

$$a^{'} \in \arg\max_{a \in A} u_1(\theta^{'}, s^{'}, a).$$

Since $u_1(\theta^{'}, s^{'}, a') > u_1(\theta^{'}; \pi^*) + 2d$ for some $d > 0$, there exists $0 < \epsilon < 1/8$ such that whenever (1) the mixture $\pi_2(\cdot|s^{'})$ assigns at least $1 - \epsilon$ probability to $a'$ and (2) $\pi$ is no further than $2\epsilon$ away from $\pi^*$ in $\ell_1$ norm, we have

$$u_1(\theta', s^{'}, \pi_2(\cdot|s^{'})) > u_1(\theta'; \pi) + d. \tag{4}$$

Let $N$ be given.

**Step 1**: **Constructing $\delta(N)$ and $\gamma(N, \delta)$.**

We will first define a series of constants.

**Step 1a**: $\underline{Q}$ and $\phi$, a bound on the fraction of "unrepresentative" samples that give senders misleading impressions of the equilibrium payoff.

As before, we will adopt notation from Fudenberg and Levine (1993).

In FL93 Lemma 5.6, take $\epsilon$ to be the $\epsilon$ from the line immediately above Equation (4). Then, there exists some $\phi > 0$ so that for any arbitrary steady state $\psi$,

$$\psi_i \left\{ y_i : Q^i_\epsilon(\bar{\psi}_{-i}|y_i)/Q^i_\epsilon(\bar{\psi}_{-i}|0) < \phi \right\} \leq \frac{1}{8}.$$

Now, if a steady state strategy profile $\bar{\psi}$ is no more than $\epsilon$ away from $\pi^*$, then the $\epsilon$-ball around $\bar{\psi}$ is inside the $2\epsilon$-ball around $\pi^*$, i.e. $B^i_\epsilon(\bar{\psi}_{-i}) \subseteq B^i_{2\epsilon}(\pi^*_{-i})$, so taking $i = \theta'$ and $-i = 2$ yields

$$\psi_{\theta'} \left\{ y_{\theta'} : Q^{\theta'}_{2\epsilon}(\pi^*_2|y_{\theta'})/Q^{\theta'}_\epsilon(\bar{\psi}_2|0) < \phi \right\} \leq \frac{1}{8}.$$

Since $g_1$ is non-doctrinaire, all $\epsilon$-balls in $\Pi_2$ must have some lower bound on their prior probability, let's say $\underline{Q}$. So

$$\psi_{\theta'} \left\{ y_{\theta'} : Q^{\theta'}_{2\epsilon}(\pi^*_2|y_{\theta'}) < \underline{Q}\phi \right\} \leq \frac{1}{8}.$$

**Step 1b**: $h$, the minimum chance of improving payoff by $d$ when $\theta'$ plays $s'$ at "representative" histories where $s'$ has not been played much before.

Let $\underline{p} > 0$ be the least possible probability placed on those receiver strategies $\pi_2$ such that $\pi_2(a'|s') > 1 - \epsilon$, after a history where $\theta'$ played $s'$ fewer than $2N$ times in the past. Write also $S_{\theta'}$ for the set of signals that $\theta'$ sends with positive probability in $\pi^*$. Then, for every history $y_{\theta'}$ such that $Q^{\theta'}_{2\epsilon}(\pi^*_2|y_{\theta'}) \geq \underline{Q}\phi$ and $\#(s'|y_{\theta'}) < 2N$, we have for every $s_{\theta'} \in S_{\theta'}$,

$$P(s_{\theta'}, d, y_{\theta'}) \geq g_1 \left\{ \pi_2 : u_1(\theta', s', \pi_2(\cdot|s')) \geq u_1(\theta', s_{\theta'}, \pi_2(\cdot|s_{\theta'})) + d|y_{\theta'} \right\} \geq \underline{Q}\phi \cdot \underline{p}.$$

In words, this says there is at least $\underline{Q}\phi\underline{p}$ chance that playing $s'$ instead of the signal $s_{\theta'}$ yields a gain of at least $d$. To see why this is true, note that if in history $y_{\theta'}$ type $\theta$ played $s'$ no more than $2N$ times before, then it must assign at least $\underline{p}$ chance to the event that receiver has a mixed strategy that responds to $s'$ with $a'$ at least $1-\epsilon$ of the time. At the same time, since $y_{\theta'}$ by construction induces a belief that assigns at least $\underline{Q}\phi$ probability to the receiver playing a strategy no more than $2\epsilon$ away from $\pi^*_2(\cdot|s')$ after signal $s'$, by (4) the probability assigned to receiver strategies against which $s'$ improves on $s_{\theta'}$ by at least $d$ is at least $\underline{Q}\phi \cdot \underline{p}$. (We can multiply here since the prior over receiver strategy is independent.) Let $h \coloneqq \underline{Q}\phi \cdot \underline{p}$ denote this minimum probability.

**Step 1c**: $\underline{\beta}$, the minimum effective discount factor required to realize the gain of $hd$ through a statistical test.

In FL93 Lemma 5.3, let $\Delta = d$ and let $\epsilon$ be small enough such that $(1-\epsilon) \cdot (hd - \epsilon) > \frac{hd}{2}$.

This gives rise to a $\underline{\beta}$, such that whenever $\delta\gamma > \underline{\beta}$,

$$V_{\theta'}(y_{\theta'}) - u_{\theta'}(\sigma_{\theta'}(y_{\theta'})|y_{\theta'}) > \frac{hd}{2}$$

at every history $y_{\theta'}$ where $P(\sigma_{\theta'}(y_{\theta'}), d, y_{\theta'}) > h$.

**Step 1d**: $N(\delta)$, the number of times the current strategy needs to be played before option value becomes negligible.

For each $\delta$, substitute $\epsilon = \frac{\frac{1}{2}hd}{\delta/(1-\delta)}$ in the statement of FL93 Corollary 5.5. This leads to some number $N(\delta)$, such that if $\theta'$ has played what she intends to play in the current period at least $N(\delta)$ times, then there is probability no larger than $\frac{\frac{1}{2}hd}{\delta/(1-\delta)}$ that the option value of $y_i$ exceeds $\frac{1}{2}hd$. (This is uniform for all $\gamma$ since for every $\gamma \in (0,1)$, $\frac{\delta\gamma}{1-\delta\gamma} < \frac{\delta}{1-\delta}$, so the corollary actually gives a tighter bound than just stated.)

**Step 1e**: Finally, we define $\delta(N)$ and $\gamma(N,\delta)$.

Choose $\delta(N)$ large enough so that (i) $\delta(N) > \sqrt{\underline{\beta}}$ from Step 1c, and (ii) $\frac{\frac{1}{2}hd}{\delta(N)/(1-\delta(N))} < \frac{1}{8}$ from step 1d.

Choose $\gamma(N,\delta)$ close enough to 1 so that (i) histories at which a player plays some strategy that she has played before $N(\delta)$ times or fewer have probability less than 1/8, (ii) $\gamma(N,\delta) > \sqrt{\underline{\beta}}$ from Step 1c.

**Step 2**: **At most histories, $\theta'$ has played $m'$ at least $2N$ times in the past.**

We consider four subsets of $Y_{\theta'}$, called $E_1, E_2, E_3, E_4$, which are "exceptional histories". We argue that whenever the hypotheses of the proposition hold, $\psi_{\theta'}(E_j) < 1/8$ for $1 \le j \le 4$ and furthermore, for any history $y_{\theta'} \notin E_1 \cup E_2 \cup E_3 \cup E_4$, we have $\#(s'|y_{\theta'}) \ge 2N$.

**Exception 1**: $\theta'$ does not play a signal associated with $\pi^*$. That is, $E_1 := \{y_{\theta'} : \sigma_{\theta'}(y_{\theta'}) \notin S_{\theta'}\}$. But since $\bar{\psi}_1(\cdot|\theta)$ is no more than $\epsilon$ away from $\pi_1^*(\cdot|\theta')$ and $\epsilon < 1/8$, we must get $\psi_{\theta'}(E_1) < 1/8$.

**Exception 2**: $\theta'$ plays an equilibrium signal, but it has played that signal fewer than $N(\delta)$ times before. That is,

$$E_2 := \{y_{\theta'} : \sigma_{\theta'}(y_{\theta'}) \in S_{\theta'}, \#(\sigma_{\theta'}(y_{\theta'})|y_{\theta'}) < N(\delta)\}.$$

But since $\gamma \ge \gamma(N,\delta)$, by construction we get $\psi_{\theta'}(E_2) < 1/8$.

**Exception 3**: $\theta'$ has a very misleading sample as to the payoff of the equilibrium signal, that is,

$$E_3 := \left\{ y_{\theta'} : Q_{2\epsilon}^{\theta'}(\pi_2^*|y_{\theta'}) < \underline{Q}\phi \right\}.$$

But by choice of of $\underline{Q}$ and $\phi$ in step 1a, $\psi_{\theta'}\{E_3\} < \frac{1}{8}$.

**Exception 4**: Special histories where $\theta'$ has a representative sample, played a signal

associated with $\pi^*$ a lot, yet still has excess option value. That is,

$$E_4 := \left\{ y_{\theta'} : V_{\theta'}(y_{\theta'}) - u_{\theta'}(\sigma_{\theta'}(y_{\theta'})|y_{\theta'}) > \frac{1}{2}hd, \text{ and } \#(\sigma_{\theta'}(y_{\theta'})|y_{\theta'}) > N(\delta) \right\}.$$

But by step 1d, $\psi_{\theta'}\{E_4\} < \frac{1}{8}$.

Now consider some history outside of these exceptions, $y_{\theta'} \notin E_1 \cup E_2 \cup E_3 \cup E_4$. The fact that $y_{\theta'} \notin E_2$ implies $\#(\sigma_{\theta'}(y_{\theta'})|y_{\theta'}) > N(\delta)$. The fact that $y_{\theta'} \notin E_4$ then implies $V_{\theta'}(y_{\theta'}) - u_{\theta'}(\sigma_{\theta'}(y_{\theta'})|y_{\theta'}) \leq \frac{1}{2}hd$. Suppose it were the case that $\#(s'|y_{\theta'}) < 2N$. Then $y_{\theta'} \notin E_1$ implies $\sigma_{\theta'}(y_{\theta'}) \in S_{\theta'}$ while $y_{\theta'} \notin E_3$ implies $Q_{2\epsilon}^{\theta'}(\pi_2^*|y_{\theta'}) \geq \underline{Q}\phi$. So then by step 1b, $P(\sigma_{\theta'}(y_{\theta'}), d, y_{\theta'}) > h$. But since $\delta \cdot \gamma > \underline{\beta}$, step 1c implies that

$$V_{\theta'}(y_{\theta'}) - u_{\theta'}(\sigma_{\theta'}(y_{\theta'})|y_{\theta'}) > \frac{hd}{2},$$

which is a contradiction. Therefore it must be that $\#(s'|y_{\theta'}) \geq 2N$. That is,

$$\psi_{\theta'}\{y_{\theta'} : \#(s'|y_{\theta'}) \geq 2N\} \geq \frac{1}{2}.$$

**Step 3**: **Bounding the probability of histories where $\theta'$ plays $s'$.**

We know that at most histories type $\theta'$ has played $s'$ at least $2N$ times in the past, but we are after a bound on those histories where $\theta'$ plays $s'$ in the current period. Towards that end, we introduce some new notation: for two histories of type $\theta'$, say $y^1$ and $y^2$, write $y^1 \lessdot y^2$ if $y^2$ is a strict continuation of $y^1$ – that is, $y^2$ is $y^1$ concatenated with one or more additional periods of experience at the end. We state a lemma below (with proof independent of this proposition), that says the probability of any history $y^1$ in the learning model is no less than the sum of probabilities of any collection of its continuations that "avoids double counting."

Consider the set of histories $Y_{\theta'}^{\text{first}} \subseteq Y_{\theta'}$ given by

$$Y_{\theta'}^{\text{first}} := \{y_{\theta'} : \#(s'|y_{\theta'}) = 2N \text{ and } \#(s'|y'_{\theta'}) < 2N \text{ for any } y'_{\theta'} \lessdot y_{\theta'}\},$$

that is, the set of earliest histories where $\theta'$ has sent signal $s'$ for $2N$ times in the past. It is easy to see that no two members of $Y_{\theta'}^{\text{first}}$ are strict continuations of each other.

If $y_{\theta'} \in Y_{\theta'}^{\text{first}}$, then for every strict continuation $y_{\theta'} \lessdot y'_{\theta'}$ we have $\#(s'|y'_{\theta'}) \geq 2N$. But the set of all continuations of $y_{\theta'}$ plus $y_{\theta'}$ itself have mass $\psi_{\theta'}(y_{\theta'})/(1-\gamma)$ under steady state $\psi$ , so we get

$$\psi_{\theta'}\{y_{\theta'} : \#(s'|y_{\theta'}) \geq 2N\} = \sum_{y_{\theta'} \in Y_{\theta'}^{\text{first}}} \psi_{\theta'}(y_{\theta'})/(1-\gamma) \geq \frac{1}{2},$$

where the inequality comes from step 2. But now for each $y_{\theta'}^*$ such that $\sigma_{\theta'}(y_{\theta'}^*) = s'$, we

may consider the subset of $Y_{\theta'}^{\text{first}}$ which are strict continuations of $y_{\theta'}^*$, which we will denote by $Y_{\theta'}^{\text{first}}[y_{\theta'}^*]$. Then by Lemma OA.4,

$$\sum_{y_{\theta'}^*:\sigma_{\theta'}(y_{\theta'}^*)=s'} \psi_{\theta'}(y_{\theta'}^*) \geq \sum_{y_{\theta'}^*:\sigma_{\theta'}(y_{\theta'}^*)=s'} \left( \sum_{y_{\theta'} \in Y_{\theta'}^{\text{first}}[y_{\theta'}^*]} \psi_{\theta'}(y_{\theta'}) \right).$$

But for each $y_{\theta'} \in Y_{\theta'}^{\text{first}}$, there are exactly $2N$ histories $y_{\theta'}^*$ where $\sigma_{\theta'}(y_{\theta'}^*) = s'$ for which $y_{\theta'}$ is a strict continuation, that is, $y_{\theta'}$ belongs to exactly $2N$ of the $Y_{\theta'}^{\text{first}}[y_{\theta'}^*]$ sets.

Thus we can rewrite the RHS as

$$\sum_{y_{\theta'}^*:\sigma_{\theta'}(y_{\theta'}^*)=s'} \left( \sum_{y_{\theta'} \in Y_{\theta'}^{\text{first}}[y_{\theta'}^*]} \psi_{\theta'}(y_{\theta'}) \right) = 2N \cdot \sum_{y_{\theta'} \in Y_{\theta'}^{\text{first}}} \psi_{\theta'}(y_{\theta'}) \geq 2N \cdot \frac{1}{2} \cdot (1-\gamma) = N(1-\gamma).$$

So

$$\sum_{y_{\theta'}^*:\sigma_{\theta'}(y_{\theta'}^*)=s'} \psi_{\theta'}(y_{\theta'}^*) \geq N(1-\gamma),$$

as desired. □

**Lemma OA.4.** In any steady state $\psi$ and for any player $i$, suppose $y_i^*$ is some finite history and $C$ is a collection of histories such that (i) $y_i^* \lessdot y_i$ for all $y_i \in C$, and (ii) there are no two $y_i', y_i'' \in C$ with $y_i' \lessdot y_i''$. Then $\psi_i(y_i^*) \geq \sum_{y_i \in C} \psi_i(y_i)$. (Here, the notation $y_i^* \lessdot y_i$ means history $y_i$ is a strict continuation of history $y_i^*$.)

*Proof.* We first show the statement is true if the maximal length of histories in $C$ is bounded by length of $y_i^*$ plus $t$, for every $t \in \mathbb{N}$. The base case of $t = 1$ is evident since the set of all continuations of $y_i^*$ with one additional period of experience have probability $\psi_i(y_i^*) \cdot \gamma \leq \psi_i(y_i^*)$. Now suppose this statement is true whenever $t \leq T$. To prove the case of $t = T + 1$, write $\hat{D}$ for the set of all one-period continuation of $y_i^*$, and observe for each $\hat{y}_i \in \hat{D}$, by the inductive hypothesis,

$$\psi_i(\hat{y}_i) \geq \sum_{y_i \in C_{\hat{y}_i}} \psi_i(y_i)$$

where $C_{\hat{y}_i} \subseteq C$ is the subset of $C$ which are strict continuations of $\hat{y}_i$. Observe also whenever $\hat{y}_i \in C$, we get $C_{\hat{y}_i} = \emptyset$, else we would have two continuations of $y_i^*$ both in $C$ which are strict continuations of each other. As such, we conclude

$$\psi_i(y_i^*) \geq \sum_{\hat{y}_i \in \hat{D}} \psi_i(\hat{y}_i) \geq \left( \sum_{\hat{y}_i \in C} \psi_i(\hat{y}_i) \right) + \sum_{\hat{y}_i \notin C} \left( \sum_{y_i \in C_{\hat{y}_i}} \psi_i(y_i) \right) = \sum_{y_i \in C} \psi_i(y_i)$$

as desired.

But if the statement holds when $C$ is restricted to histories that continue $y_i^*$ for no more than $t$ periods for every $t \in \mathbb{N}$, then it must also hold for all of $C$, since the probability assigned to histories with length greater than $T$ vanishes with $T \to \infty$. $\square$

# References

Aliprantis, C. D. and K. C. Border (2006): *Infinite Dimensional Analysis: A Hitchhiker's Guide*, Springer.

Fudenberg, D. and D. K. Levine (1993): "Steady State Learning and Nash Equilibrium," *Econometrica*, 61, 547–573.
